# Supplementary material for: Evolution of World Running Record Performances for Men and Women: Physiological Characteristics
Source: arXiv:2401.09171 source file (2024-01-17)
Supplement: Supplementary file 1 [file WR_SupplementaryMaterial.pdf]

## ***Supplementary Material***

Below we provide tables for the analyzed WR data for men and women. For each year, the tables give the fitted model parameters, and for each distance the actual WR times (1st line), the model estimated times (2nd line), and the relative error in percent (3rd line). Also given is the average error for all distances in percent, and the WRs and predicted times for the half and full marathon.

Magenta color indicates a new WR in the given year. Red (green) color marks the slowest (fastest) time relative to the model fit.

# World Records Men

| Year | t <sub>c</sub> | v <sub>m</sub> [m/min] | E <sub>s</sub> | E <sub>l</sub> | Y <sub>an</sub> | Y <sub>ae</sub> | 1000                          | 1500                          | 1609.34                       | 2000                          | 3000                          | 5000                          | 10 000                        | av.err[%] | Halfmarathon | Marathon                          |
|------|----------------|------------------------|----------------|----------------|-----------------|-----------------|-------------------------------|-------------------------------|-------------------------------|-------------------------------|-------------------------------|-------------------------------|-------------------------------|-----------|--------------|-----------------------------------|
| 1918 | 06:26.51       | 358.27                 | 0.48           | 5.06           | 0.135           | 0.062           | 02:29.10<br>02:28.34<br>-0.51 | 03:54.70<br>03:55.49<br>0.34  | 04:12.60<br>04:15.25<br>1.05  | 05:30.40<br>05:27.65<br>-0.83 | 08:33.20<br>08:31.23<br>-0.38 | 14:36.60<br>14:42.28<br>0.65  | 30:58.80<br>30:54.09<br>-0.25 | 0.57      | 1:08:58.72   | 2:36:06.60<br>2:25:51.08<br>-6.57 |
| 1919 | 06:26.51       | 358.27                 | 0.48           | 5.06           | 0.135           | 0.062           | 02:29.10<br>02:28.34<br>-0.51 | 03:54.70<br>03:55.49<br>0.34  | 04:12.60<br>04:15.25<br>1.05  | 05:30.40<br>05:27.65<br>-0.83 | 08:33.20<br>08:31.23<br>-0.38 | 14:36.60<br>14:42.28<br>0.65  | 30:58.80<br>30:54.09<br>-0.25 | 0.57      | 1:08:58.72   | 2:36:06.60<br>2:25:51.08<br>-6.57 |
| 1920 | 06:26.51       | 358.27                 | 0.48           | 5.06           | 0.135           | 0.062           | 02:29.10<br>02:28.34<br>-0.51 | 03:54.70<br>03:55.49<br>0.34  | 04:12.60<br>04:15.25<br>1.05  | 05:30.40<br>05:27.65<br>-0.83 | 08:33.20<br>08:31.23<br>-0.38 | 14:36.60<br>14:42.28<br>0.65  | 30:58.80<br>30:54.09<br>-0.25 | 0.57      | 1:08:58.72   | 2:32:35.80<br>2:25:51.08<br>-4.42 |
| 1921 | 06:43.68       | 356.18                 | 0.48           | 6.18           | 0.135           | 0.055           | 02:29.10<br>02:28.34<br>-0.51 | 03:54.70<br>03:55.49<br>0.34  | 04:12.60<br>04:15.25<br>1.05  | 05:30.40<br>05:27.65<br>-0.83 | 08:33.20<br>08:32.05<br>-0.22 | 14:36.60<br>14:39.92<br>0.38  | 30:40.20<br>30:37.42<br>-0.15 | 0.50      | 1:07:50.35   | 2:32:35.80<br>2:22:18.41<br>-6.74 |
| 1922 | 06:42.91       | 359.20                 | 0.45           | 5.22           | 0.126           | 0.061           | 02:28.60<br>02:28.35<br>-0.17 | 03:54.70<br>03:54.56<br>-0.06 | 04:12.60<br>04:14.05<br>0.57  | 05:26.40<br>05:25.30<br>-0.34 | 08:28.60<br>08:28.26<br>-0.07 | 14:35.40<br>14:36.39<br>0.11  | 30:40.20<br>30:39.36<br>-0.05 | 0.20      | 1:08:19.47   | 2:32:35.80<br>2:24:14.00<br>-5.48 |
| 1923 | 07:00.96       | 358.25                 | 0.45           | 5.20           | 0.125           | 0.061           | 02:28.60<br>02:28.15<br>-0.30 | 03:54.70<br>03:54.06<br>-0.27 | 04:10.40<br>04:13.47<br>1.23  | 05:26.40<br>05:24.40<br>-0.61 | 08:28.60<br>08:28.26<br>-0.07 | 14:35.40<br>14:36.39<br>0.11  | 30:40.20<br>30:39.36<br>-0.05 | 0.38      | 1:08:19.47   | 2:32:35.80<br>2:24:14.00<br>-5.48 |
| 1924 | 07:24.19       | 356.56                 | 0.45           | 7.92           | 0.126           | 0.048           | 02:28.60<br>02:27.82<br>-0.52 | 03:52.60<br>03:53.53<br>0.40  | 04:10.40<br>04:12.90<br>1.00  | 05:26.40<br>05:23.66<br>-0.84 | 08:28.60<br>08:28.12<br>-0.09 | 14:28.20<br>14:29.59<br>0.16  | 30:06.20<br>30:05.03<br>-0.07 | 0.44      | 1:06:10.40   | 2:32:35.80<br>2:17:48.63<br>-9.69 |
| 1925 | 07:21.52       | 357.25                 | 0.45           | 7.52           | 0.124           | 0.050           | 02:28.60<br>02:27.87<br>-0.49 | 03:52.60<br>03:53.46<br>0.37  | 04:10.40<br>04:12.79<br>0.95  | 05:26.00<br>05:23.40<br>-0.80 | 08:27.60<br>08:27.35<br>-0.05 | 14:28.20<br>14:28.92<br>0.08  | 30:06.20<br>30:05.59<br>-0.03 | 0.40      | 1:06:16.68   | 2:29:01.80<br>2:18:12.43<br>-7.26 |
| 1926 | 05:55.40       | 366.00                 | 0.48           | 5.63           | 0.137           | 0.058           | 02:26.80<br>02:26.11<br>-0.47 | 03:51.00<br>03:52.35<br>0.58  | 04:10.40<br>04:11.93<br>0.61  | 05:26.00<br>05:23.72<br>-0.70 | 08:20.40<br>08:21.82<br>0.28  | 14:28.20<br>14:24.08<br>-0.47 | 30:06.20<br>30:09.77<br>0.20  | 0.47      | 1:07:03.48   | 2:29:01.80<br>2:21:11.49<br>-5.26 |
| 1927 | 06:09.69       | 365.17                 | 0.49           | 5.61           | 0.138           | 0.058           | 02:25.80<br>02:25.55<br>-0.17 | 03:51.00<br>03:51.48<br>0.21  | 04:10.40<br>04:10.99<br>0.24  | 05:23.40<br>05:22.53<br>-0.27 | 08:20.40<br>08:21.82<br>0.28  | 14:28.20<br>14:24.08<br>-0.47 | 30:06.20<br>30:09.77<br>0.20  | 0.26      | 1:07:03.48   | 2:29:01.80<br>2:21:11.49<br>-5.26 |
| 1928 | 06:09.69       | 365.17                 | 0.49           | 5.61           | 0.138           | 0.058           | 02:25.80<br>02:25.55<br>-0.17 | 03:51.00<br>03:51.48<br>0.21  | 04:10.40<br>04:10.99<br>0.24  | 05:23.40<br>05:22.53<br>-0.27 | 08:20.40<br>08:21.82<br>0.28  | 14:28.20<br>14:24.08<br>-0.47 | 30:06.20<br>30:09.77<br>0.20  | 0.26      | 1:07:03.48   | 2:29:01.80<br>2:21:11.49<br>-5.26 |
| 1929 | 06:09.69       | 365.17                 | 0.49           | 5.61           | 0.138           | 0.058           | 02:25.80<br>02:25.55<br>-0.17 | 03:51.00<br>03:51.48<br>0.21  | 04:10.40<br>04:10.99<br>0.24  | 05:23.40<br>05:22.53<br>-0.27 | 08:20.40<br>08:21.82<br>0.28  | 14:28.20<br>14:24.08<br>-0.47 | 30:06.20<br>30:09.77<br>0.20  | 0.26      | 1:07:03.48   | 2:29:01.80<br>2:21:11.49<br>-5.26 |
| 1930 | 05:55.06       | 366.02                 | 0.53           | 5.63           | 0.158           | 0.058           | 02:23.60<br>02:23.42<br>-0.13 | 03:49.20<br>03:50.15<br>0.41  | 04:10.40<br>04:09.98<br>-0.17 | 05:23.40<br>05:23.03<br>-0.11 | 08:20.40<br>08:21.82<br>0.28  | 14:28.20<br>14:24.08<br>-0.47 | 30:06.20<br>30:09.77<br>0.20  | 0.25      | 1:07:03.48   | 2:29:01.80<br>2:21:11.49<br>-5.26 |
| 1931 | 06:13.33       | 364.96                 | 0.52           | 5.60           | 0.152           | 0.058           | 02:23.60<br>02:23.49<br>-0.08 | 03:49.20<br>03:49.59<br>0.17  | 04:09.20<br>04:09.23<br>0.01  | 05:21.80<br>05:21.48<br>-0.10 | 08:20.40<br>08:21.82<br>0.28  | 14:28.20<br>14:24.08<br>-0.47 | 30:06.20<br>30:09.77<br>0.20  | 0.19      | 1:07:03.48   | 2:29:01.80<br>2:21:11.49<br>-5.26 |
| 1932 | 05:41.92       | 369.85                 | 0.51           | 5.20           | 0.150           | 0.061           | 02:23.60<br>02:23.49<br>-0.08 | 03:49.20<br>03:49.59<br>0.17  | 04:09.20<br>04:09.23<br>0.01  | 05:21.80<br>05:21.48<br>-0.10 | 08:18.80<br>08:18.05<br>-0.15 | 14:17.00<br>14:19.17<br>0.25  | 30:06.20<br>30:04.37<br>-0.10 | 0.12      | 1:07:04.64   | 2:29:01.80<br>2:21:43.02<br>-4.91 |
| 1933 | 05:50.22       | 369.31                 | 0.51           | 5.19           | 0.149           | 0.061           | 02:23.60<br>02:23.33<br>-0.19 | 03:49.00<br>03:49.17<br>0.07  | 04:07.60<br>04:08.74<br>0.46  | 05:21.80<br>05:20.71<br>-0.34 | 08:18.80<br>08:18.05<br>-0.15 | 14:17.00<br>14:19.17<br>0.25  | 30:06.20<br>30:04.37<br>-0.10 | 0.22      | 1:07:04.64   | 2:29:01.80<br>2:21:43.02<br>-4.91 |
| 1934 | 05:51.82       | 369.48                 | 0.51           | 5.12           | 0.149           | 0.061           | 02:23.60<br>02:23.23<br>-0.26 | 03:48.80<br>03:48.94<br>0.06  | 04:06.80<br>04:08.47<br>0.68  | 05:21.80<br>05:20.30<br>-0.47 | 08:18.40<br>08:17.74<br>-0.13 | 14:17.00<br>14:18.90<br>0.22  | 30:06.20<br>30:04.60<br>-0.09 | 0.27      | 1:07:07.31   | 2:29:01.80<br>2:21:53.44<br>-4.79 |

| Year | t <sub>c</sub> | v <sub>m</sub> [m/min] | E <sub>s</sub> | E <sub>l</sub> | Y <sub>an</sub> | Y <sub>ae</sub> | 1000                          | 1500                          | 1609.34                       | 2000                          | 3000                          | 5000                          | 10 000                        | av.err[%] | Halfmarathon | Marathon                          |
|------|----------------|------------------------|----------------|----------------|-----------------|-----------------|-------------------------------|-------------------------------|-------------------------------|-------------------------------|-------------------------------|-------------------------------|-------------------------------|-----------|--------------|-----------------------------------|
| 1935 | 05:51.82       | 369.48                 | 0.51           | 5.12           | 0.149           | 0.061           | 02:23.60<br>02:23.23<br>-0.26 | 03:48.80<br>03:48.94<br>0.06  | 04:06.80<br>04:08.47<br>0.68  | 05:21.80<br>05:20.30<br>-0.47 | 08:18.40<br>08:17.74<br>-0.13 | 14:17.00<br>14:18.90<br>0.22  | 30:06.20<br>30:04.60<br>-0.09 | 0.27      | 1:07:07.31   | 2:26:42.00<br>2:21:53.44<br>-3.28 |
| 1936 | 05:39.14       | 372.85                 | 0.50           | 4.62           | 0.143           | 0.065           | 02:23.60<br>02:23.22<br>-0.27 | 03:47.80<br>03:48.44<br>0.28  | 04:06.80<br>04:07.83<br>0.42  | 05:20.40<br>05:19.05<br>-0.42 | 08:14.80<br>08:14.99<br>0.04  | 14:17.00<br>14:16.44<br>-0.07 | 30:06.20<br>30:06.68<br>0.03  | 0.22      | 1:07:31.67   | 2:26:42.00<br>2:23:29.31<br>-2.19 |
| 1937 | 06:20.54       | 370.01                 | 0.47           | 4.59           | 0.133           | 0.066           | 02:23.60<br>02:23.56<br>-0.03 | 03:47.80<br>03:47.70<br>-0.05 | 04:06.40<br>04:06.76<br>0.15  | 05:16.80<br>05:16.57<br>-0.07 | 08:14.80<br>08:15.02<br>0.04  | 14:17.00<br>14:16.37<br>-0.07 | 30:05.60<br>30:06.14<br>0.03  | 0.06      | 1:07:29.43   | 2:26:42.00<br>2:23:22.20<br>-2.27 |
| 1938 | 06:24.15       | 369.54                 | 0.47           | 4.73           | 0.133           | 0.064           | 02:23.60<br>02:23.56<br>-0.03 | 03:47.80<br>03:47.70<br>-0.05 | 04:06.40<br>04:06.76<br>0.15  | 05:16.80<br>05:16.57<br>-0.07 | 08:14.80<br>08:15.17<br>0.08  | 14:17.00<br>14:15.92<br>-0.13 | 30:02.00<br>30:02.92<br>0.05  | 0.08      | 1:07:16.03   | 2:26:42.00<br>2:22:39.77<br>-2.75 |
| 1939 | 06:13.19       | 370.97                 | 0.47           | 5.08           | 0.133           | 0.061           | 02:23.60<br>02:23.56<br>-0.03 | 03:47.80<br>03:47.70<br>-0.05 | 04:06.40<br>04:06.76<br>0.15  | 05:16.80<br>05:16.57<br>-0.07 | 08:14.80<br>08:13.71<br>-0.22 | 14:08.80<br>14:11.94<br>0.37  | 29:52.60<br>29:49.97<br>-0.15 | 0.15      | 1:06:34.62   | 2:26:42.00<br>2:20:44.28<br>-4.06 |
| 1940 | 05:16.80       | 379.03                 | 0.46           | 4.39           | 0.130           | 0.068           | 02:23.60<br>02:23.56<br>-0.03 | 03:47.80<br>03:47.69<br>-0.05 | 04:06.40<br>04:06.76<br>0.15  | 05:16.80<br>05:16.57<br>-0.07 | 08:09.00<br>08:09.29<br>0.06  | 14:08.80<br>14:07.98<br>-0.10 | 29:52.60<br>29:53.30<br>0.04  | 0.07      | 1:07:14.02   | 2:26:42.00<br>2:23:19.95<br>-2.30 |
| 1941 | 04:55.94       | 380.62                 | 0.52           | 4.44           | 0.154           | 0.067           | 02:21.50<br>02:21.54<br>0.03  | 03:47.60<br>03:47.19<br>-0.18 | 04:06.40<br>04:06.78<br>0.15  | 05:16.80<br>05:16.71<br>-0.03 | 08:09.00<br>08:09.42<br>0.09  | 14:08.80<br>14:08.08<br>-0.08 | 29:52.60<br>29:53.07<br>0.03  | 0.08      | 1:07:12.30   | 2:26:42.00<br>2:23:13.52<br>-2.37 |
| 1942 | 04:21.74       | 390.90                 | 0.48           | 3.86           | 0.138           | 0.074           | 02:21.50<br>02:21.52<br>0.01  | 03:45.80<br>03:45.63<br>-0.08 | 04:04.60<br>04:04.76<br>0.07  | 05:11.80<br>05:10.95<br>-0.27 | 08:01.20<br>08:02.30<br>0.23  | 13:58.20<br>13:59.98<br>0.21  | 29:52.60<br>29:49.67<br>-0.16 | 0.15      | 1:07:43.44   | 2:26:42.00<br>2:25:50.60<br>-0.58 |
| 1943 | 04:56.55       | 387.29                 | 0.46           | 3.81           | 0.128           | 0.075           | 02:21.50<br>02:21.56<br>0.04  | 03:45.00<br>03:44.40<br>-0.27 | 04:02.60<br>04:03.16<br>0.23  | 05:11.80<br>05:10.95<br>-0.27 | 08:01.20<br>08:02.30<br>0.23  | 13:58.20<br>13:59.98<br>0.21  | 29:52.60<br>29:49.67<br>-0.16 | 0.20      | 1:07:43.44   | 2:26:42.00<br>2:25:50.60<br>-0.58 |
| 1944 | 05:17.35       | 385.21                 | 0.46           | 4.05           | 0.128           | 0.072           | 02:21.50<br>02:21.17<br>-0.23 | 03:43.00<br>03:43.66<br>0.29  | 04:01.60<br>04:02.33<br>0.30  | 05:11.80<br>05:10.68<br>-0.36 | 08:01.20<br>08:01.66<br>0.10  | 13:58.20<br>13:56.86<br>-0.16 | 29:35.40<br>29:36.54<br>0.06  | 0.22      | 1:06:55.26   | 2:26:42.00<br>2:23:23.76<br>-2.25 |
| 1945 | 05:18.74       | 385.09                 | 0.46           | 4.04           | 0.127           | 0.072           | 02:21.50<br>02:21.15<br>-0.24 | 03:43.00<br>03:43.61<br>0.27  | 04:01.40<br>04:02.28<br>0.36  | 05:11.80<br>05:10.59<br>-0.39 | 08:01.20<br>08:01.66<br>0.10  | 13:58.20<br>13:56.86<br>-0.16 | 29:35.40<br>29:36.54<br>0.06  | 0.23      | 1:06:55.26   | 2:26:42.00<br>2:23:23.76<br>-2.25 |
| 1946 | 05:17.84       | 385.16                 | 0.46           | 4.04           | 0.128           | 0.072           | 02:21.40<br>02:21.07<br>-0.23 | 03:43.00<br>03:43.57<br>0.26  | 04:01.40<br>04:02.26<br>0.35  | 05:11.80<br>05:10.64<br>-0.37 | 08:01.20<br>08:01.66<br>0.10  | 13:58.20<br>13:56.86<br>-0.16 | 29:35.40<br>29:36.54<br>0.06  | 0.22      | 1:06:55.26   | 2:26:42.00<br>2:23:23.76<br>-2.25 |
| 1947 | 05:17.84       | 385.16                 | 0.46           | 4.04           | 0.128           | 0.072           | 02:21.40<br>02:21.07<br>-0.23 | 03:43.00<br>03:43.57<br>0.26  | 04:01.40<br>04:02.26<br>0.35  | 05:11.80<br>05:10.64<br>-0.37 | 08:01.20<br>08:01.66<br>0.10  | 13:58.20<br>13:56.86<br>-0.16 | 29:35.40<br>29:36.54<br>0.06  | 0.22      | 1:06:55.26   | 2:26:42.00<br>2:23:23.76<br>-1.55 |
| 1948 | 06:36.54       | 379.07                 | 0.42           | 3.96           | 0.115           | 0.073           | 02:21.40<br>02:21.57<br>0.12  | 03:43.00<br>03:42.69<br>-0.14 | 04:01.40<br>04:00.97<br>-0.18 | 05:07.00<br>05:07.61<br>0.20  | 08:01.20<br>08:01.66<br>0.10  | 13:58.20<br>13:56.86<br>-0.16 | 29:35.40<br>29:36.54<br>0.06  | 0.14      | 1:06:55.26   | 2:25:39.00<br>2:23:23.76<br>-1.55 |
| 1949 | 06:19.63       | 380.96                 | 0.42           | 4.16           | 0.114           | 0.070           | 02:21.40<br>02:21.57<br>0.12  | 03:43.00<br>03:42.69<br>-0.14 | 04:01.40<br>04:00.97<br>-0.18 | 05:07.00<br>05:07.61<br>0.20  | 07:58.80<br>08:00.43<br>0.34  | 13:58.20<br>13:53.47<br>-0.56 | 29:21.20<br>29:25.32<br>0.23  | 0.25      | 1:06:18.63   | 2:25:39.00<br>2:21:39.22<br>-2.74 |
| 1950 | 06:44.18       | 378.24                 | 0.42           | 4.84           | 0.115           | 0.063           | 02:21.40<br>02:21.57<br>0.12  | 03:43.00<br>03:42.69<br>-0.14 | 04:01.40<br>04:00.97<br>-0.18 | 05:07.00<br>05:07.61<br>0.20  | 07:58.80<br>08:01.22<br>0.50  | 13:58.20<br>13:51.16<br>-0.84 | 29:02.60<br>29:08.79<br>0.36  | 0.33      | 1:05:09.44   | 2:25:39.00<br>2:17:59.19<br>-5.26 |
| 1951 | 06:44.18       | 378.24                 | 0.42           | 4.84           | 0.115           | 0.063           | 02:21.40<br>02:21.57<br>0.12  | 03:43.00<br>03:42.69<br>-0.14 | 04:01.40<br>04:00.97<br>-0.18 | 05:07.00<br>05:07.61<br>0.20  | 07:58.80<br>08:01.22<br>0.50  | 13:58.20<br>13:51.16<br>-0.84 | 29:02.60<br>29:08.79<br>0.36  | 0.33      | 1:05:09.44   | 2:25:39.00<br>2:17:59.19<br>-5.26 |

| Year | t <sub>c</sub> | v <sub>m</sub> [m/min] | E <sub>s</sub> | E <sub>l</sub> | Y <sub>an</sub> | Y <sub>ae</sub> | 1000                          | 1500                          | 1609.34                       | 2000                          | 3000                          | 5000                          | 10 000                        | av.err[%] | Halfmarathon | Marathon                          |
|------|----------------|------------------------|----------------|----------------|-----------------|-----------------|-------------------------------|-------------------------------|-------------------------------|-------------------------------|-------------------------------|-------------------------------|-------------------------------|-----------|--------------|-----------------------------------|
| 1952 | 06:37.95       | 378.61                 | 0.42           | 4.85           | 0.117           | 0.063           | 02:21.20<br>02:21.40<br>0.14  | 03:43.00<br>03:42.62<br>-0.17 | 04:01.40<br>04:00.93<br>-0.20 | 05:07.00<br>05:07.71<br>0.23  | 07:58.80<br>08:01.22<br>0.50  | 13:58.20<br>13:51.16<br>-0.84 | 29:02.60<br>29:08.79<br>0.36  | 0.35      | 1:05:09.44   | 2:20:42.20<br>2:17:59.19<br>-1.93 |
| 1953 | 06:18.77       | 379.73                 | 0.45           | 4.92           | 0.124           | 0.063           | 02:20.40<br>02:20.71<br>0.22  | 03:43.00<br>03:42.31<br>-0.31 | 04:01.40<br>04:00.75<br>-0.27 | 05:07.00<br>05:08.12<br>0.36  | 07:58.80<br>08:01.26<br>0.51  | 13:58.20<br>13:51.04<br>-0.85 | 29:01.60<br>29:07.91<br>0.36  | 0.41      | 1:05:05.77   | 2:18:34.80<br>2:17:47.62<br>-0.57 |
| 1954 | 06:25.61       | 380.04                 | 0.46           | 5.21           | 0.130           | 0.061           | 02:19.50<br>02:19.50<br>0.00  | 03:41.80<br>03:40.87<br>-0.42 | 03:58.00<br>03:59.29<br>0.54  | 05:07.00<br>05:06.65<br>-0.11 | 07:58.80<br>08:00.00<br>0.25  | 13:51.20<br>13:47.70<br>-0.42 | 28:54.20<br>28:57.23<br>0.17  | 0.27      | 1:04:32.02   | 2:17:39.40<br>2:16:14.25<br>-1.03 |
| 1955 | 06:34.83       | 383.49                 | 0.43           | 4.58           | 0.117           | 0.066           | 02:19.00<br>02:19.41<br>0.29  | 03:40.80<br>03:39.55<br>-0.57 | 03:58.00<br>03:57.62<br>-0.16 | 05:02.20<br>05:03.54<br>0.44  | 07:55.60<br>07:55.15<br>-0.09 | 13:40.60<br>13:41.90<br>0.16  | 28:54.20<br>28:53.10<br>-0.06 | 0.25      | 1:04:44.78   | 2:17:39.40<br>2:17:30.38<br>-0.11 |
| 1956 | 06:16.82       | 385.68                 | 0.42           | 5.28           | 0.117           | 0.060           | 02:19.00<br>02:19.38<br>0.27  | 03:40.60<br>03:39.50<br>-0.50 | 03:58.00<br>03:57.56<br>-0.18 | 05:02.20<br>05:03.46<br>0.42  | 07:52.80<br>07:53.18<br>0.08  | 13:36.80<br>13:35.70<br>-0.13 | 28:30.40<br>28:31.34<br>0.05  | 0.23      | 1:03:32.42   | 2:17:39.40<br>2:14:04.22<br>-2.61 |
| 1957 | 06:38.33       | 384.72                 | 0.42           | 5.22           | 0.116           | 0.060           | 02:19.00<br>02:18.94<br>-0.04 | 03:38.10<br>03:38.69<br>0.27  | 03:57.20<br>03:56.66<br>-0.23 | 05:02.20<br>05:02.21<br>0.00  | 07:52.80<br>07:52.77<br>-0.01 | 13:35.00<br>13:35.09<br>0.01  | 28:30.40<br>28:30.33<br>-0.00 | 0.08      | 1:03:30.91   | 2:17:39.40<br>2:14:02.69<br>-2.62 |
| 1958 | 06:55.35       | 383.75                 | 0.44           | 5.20           | 0.123           | 0.061           | 02:18.10<br>02:17.63<br>-0.34 | 03:36.00<br>03:37.19<br>0.55  | 03:54.50<br>03:55.15<br>0.28  | 05:02.20<br>05:00.75<br>-0.48 | 07:52.80<br>07:52.77<br>-0.01 | 13:35.00<br>13:35.09<br>0.01  | 28:30.40<br>28:30.33<br>-0.00 | 0.24      | 1:03:30.91   | 2:15:17.00<br>2:14:02.69<br>-0.92 |
| 1959 | 06:46.65       | 384.24                 | 0.45           | 5.21           | 0.126           | 0.061           | 02:17.80<br>02:17.38<br>-0.30 | 03:36.00<br>03:37.07<br>0.50  | 03:54.50<br>03:55.08<br>0.25  | 05:02.20<br>05:00.89<br>-0.43 | 07:52.80<br>07:52.77<br>-0.01 | 13:35.00<br>13:35.09<br>0.01  | 28:30.40<br>28:30.33<br>-0.00 | 0.21      | 1:03:30.91   | 2:15:17.00<br>2:14:02.69<br>-0.92 |
| 1960 | 06:33.21       | 384.30                 | 0.48           | 6.02           | 0.137           | 0.056           | 02:16.70<br>02:16.39<br>-0.22 | 03:35.60<br>03:36.54<br>0.44  | 03:54.50<br>03:54.72<br>0.09  | 05:02.20<br>05:01.30<br>-0.30 | 07:52.80<br>07:53.28<br>0.10  | 13:35.00<br>13:33.62<br>-0.17 | 28:18.80<br>28:19.98<br>0.07  | 0.20      | 1:02:48.57   | 2:15:16.20<br>2:11:51.15<br>-2.53 |
| 1961 | 06:33.21       | 384.30                 | 0.48           | 6.02           | 0.137           | 0.056           | 02:16.70<br>02:16.39<br>-0.22 | 03:35.60<br>03:36.54<br>0.44  | 03:54.50<br>03:54.72<br>0.09  | 05:02.20<br>05:01.30<br>-0.30 | 07:52.80<br>07:53.28<br>0.10  | 13:35.00<br>13:33.62<br>-0.17 | 28:18.80<br>28:19.98<br>0.07  | 0.20      | 1:02:48.57   | 2:15:16.20<br>2:11:51.15<br>-2.53 |
| 1962 | 06:10.19       | 388.12                 | 0.47           | 5.30           | 0.133           | 0.060           | 02:16.70<br>02:16.45<br>-0.18 | 03:35.60<br>03:36.41<br>0.38  | 03:54.40<br>03:54.53<br>0.05  | 05:01.60<br>05:00.87<br>-0.24 | 07:49.20<br>07:50.54<br>0.29  | 13:35.00<br>13:31.11<br>-0.48 | 28:18.20<br>28:21.57<br>0.20  | 0.26      | 1:03:10.31   | 2:15:16.20<br>2:13:16.80<br>-1.47 |
| 1963 | 06:12.58       | 387.79                 | 0.47           | 5.45           | 0.133           | 0.059           | 02:16.70<br>02:16.45<br>-0.18 | 03:35.60<br>03:36.41<br>0.38  | 03:54.40<br>03:54.53<br>0.05  | 05:01.60<br>05:00.87<br>-0.24 | 07:49.20<br>07:50.65<br>0.31  | 13:35.00<br>13:30.78<br>-0.52 | 28:15.60<br>28:19.26<br>0.22  | 0.27      | 1:03:00.82   | 2:14:28.00<br>2:12:47.20<br>-1.25 |
| 1964 | 06:13.50       | 387.74                 | 0.47           | 5.45           | 0.134           | 0.059           | 02:16.60<br>02:16.34<br>-0.19 | 03:35.60<br>03:36.29<br>0.32  | 03:54.04<br>03:54.41<br>0.16  | 05:01.60<br>05:00.76<br>-0.28 | 07:49.20<br>07:50.65<br>0.31  | 13:35.00<br>13:30.78<br>-0.52 | 28:15.60<br>28:19.26<br>0.22  | 0.28      | 1:03:00.82   | 2:12:11.20<br>2:12:47.20<br>0.45  |
| 1965 | 05:02.11       | 399.04                 | 0.47           | 5.71           | 0.132           | 0.057           | 02:16.20<br>02:16.01<br>-0.14 | 03:35.60<br>03:35.95<br>0.16  | 03:53.60<br>03:54.09<br>0.21  | 05:01.20<br>05:00.51<br>-0.23 | 07:39.60<br>07:42.38<br>0.61  | 13:24.20<br>13:16.09<br>-1.01 | 27:39.89<br>27:47.08<br>0.43  | 0.40      | 1:01:45.49   | 2:12:00.00<br>2:10:00.30<br>-1.51 |
| 1966 | 05:54.01       | 396.85                 | 0.42           | 5.51           | 0.114           | 0.059           | 02:16.20<br>02:16.33<br>0.10  | 03:35.60<br>03:34.51<br>-0.50 | 03:51.30<br>03:52.13<br>0.36  | 04:56.20<br>04:56.36<br>0.06  | 07:39.60<br>07:40.68<br>0.23  | 13:16.60<br>13:13.47<br>-0.39 | 27:39.89<br>27:42.59<br>0.16  | 0.26      | 1:01:38.17   | 2:12:00.00<br>2:09:50.74<br>-1.63 |
| 1967 | 06:13.82       | 395.59                 | 0.42           | 5.48           | 0.114           | 0.059           | 02:16.20<br>02:15.94<br>-0.19 | 03:33.10<br>03:33.84<br>0.35  | 03:51.10<br>03:51.39<br>0.13  | 04:56.20<br>04:55.39<br>-0.28 | 07:39.60<br>07:40.68<br>0.23  | 13:16.60<br>13:13.47<br>-0.39 | 27:39.89<br>27:42.59<br>0.16  | 0.25      | 1:01:38.17   | 2:09:36.40<br>2:09:50.74<br>0.18  |
| 1968 | 06:13.82       | 395.59                 | 0.42           | 5.48           | 0.114           | 0.059           | 02:16.20<br>02:15.94<br>-0.19 | 03:33.10<br>03:33.84<br>0.35  | 03:51.10<br>03:51.39<br>0.13  | 04:56.20<br>04:55.39<br>-0.28 | 07:39.60<br>07:40.68<br>0.23  | 13:16.60<br>13:13.47<br>-0.39 | 27:39.89<br>27:42.59<br>0.16  | 0.25      | 1:01:38.17   | 2:09:36.40<br>2:09:50.74<br>0.18  |

| Year | t <sub>c</sub> | v <sub>m</sub> [m/min] | E <sub>s</sub> | E <sub>l</sub> | Y <sub>an</sub> | Y <sub>ae</sub> | 1000                          | 1500                          | 1609.34                       | 2000                          | 3000                          | 5000                          | 10 000                        | av.err[%] | Halfmarathon                      | Marathon                          |
|------|----------------|------------------------|----------------|----------------|-----------------|-----------------|-------------------------------|-------------------------------|-------------------------------|-------------------------------|-------------------------------|-------------------------------|-------------------------------|-----------|-----------------------------------|-----------------------------------|
| 1969 | 06:13.82       | 395.59                 | 0.42           | 5.48           | 0.114           | 0.059           | 02:16.20<br>02:15.94<br>-0.19 | 03:33.10<br>03:33.84<br>0.35  | 03:51.10<br>03:51.39<br>0.13  | 04:56.20<br>04:55.39<br>-0.28 | 07:39.60<br>07:40.68<br>0.23  | 13:16.60<br>13:13.47<br>-0.39 | 27:39.89<br>27:42.59<br>0.16  | 0.25      | 1:01:38.17                        | 2:08:33.60<br>2:09:50.74<br>1.00  |
| 1970 | 06:13.82       | 395.59                 | 0.42           | 5.48           | 0.114           | 0.059           | 02:16.20<br>02:15.94<br>-0.19 | 03:33.10<br>03:33.84<br>0.35  | 03:51.10<br>03:51.39<br>0.13  | 04:56.20<br>04:55.39<br>-0.28 | 07:39.60<br>07:40.68<br>0.23  | 13:16.60<br>13:13.47<br>-0.39 | 27:39.89<br>27:42.59<br>0.16  | 0.25      | 1:01:38.17                        | 2:08:33.60<br>2:09:50.74<br>1.00  |
| 1971 | 06:13.82       | 395.59                 | 0.42           | 5.48           | 0.114           | 0.059           | 02:16.20<br>02:15.94<br>-0.19 | 03:33.10<br>03:33.84<br>0.35  | 03:51.10<br>03:51.39<br>0.13  | 04:56.20<br>04:55.39<br>-0.28 | 07:39.60<br>07:40.68<br>0.23  | 13:16.60<br>13:13.47<br>-0.39 | 27:39.89<br>27:42.59<br>0.16  | 0.25      | 1:01:38.17                        | 2:08:33.60<br>2:09:50.74<br>1.00  |
| 1972 | 05:39.03       | 400.01                 | 0.41           | 5.18           | 0.113           | 0.061           | 02:16.20<br>02:15.94<br>-0.19 | 03:33.10<br>03:33.84<br>0.35  | 03:51.10<br>03:51.39<br>0.13  | 04:56.20<br>04:55.39<br>-0.28 | 07:37.60<br>07:38.40<br>0.17  | 13:13.00<br>13:10.69<br>-0.29 | 27:38.35<br>27:40.34<br>0.12  | 0.22      | 1:01:42.77                        | 2:08:33.60<br>2:10:21.64<br>1.40  |
| 1973 | 05:45.30       | 398.94                 | 0.42           | 5.65           | 0.115           | 0.058           | 02:16.00<br>02:15.77<br>-0.17 | 03:33.10<br>03:33.76<br>0.31  | 03:51.10<br>03:51.35<br>0.11  | 04:56.20<br>04:55.48<br>-0.24 | 07:37.60<br>07:38.72<br>0.25  | 13:13.00<br>13:09.74<br>-0.41 | 27:30.80<br>27:33.62<br>0.17  | 0.24      | 1:01:15.16                        | 2:08:33.60<br>2:08:55.55<br>0.28  |
| 1974 | 05:01.83       | 404.11                 | 0.48           | 5.23           | 0.134           | 0.060           | 02:13.90<br>02:13.84<br>-0.04 | 03:32.16<br>03:32.71<br>0.26  | 03:51.10<br>03:50.60<br>-0.21 | 04:56.20<br>04:56.20<br>0.00  | 07:35.20<br>07:36.88<br>0.37  | 13:13.00<br>13:08.12<br>-0.62 | 27:30.80<br>27:35.06<br>0.26  | 0.25      | 1:01:31.34                        | 2:08:33.60<br>2:09:58.26<br>1.10  |
| 1975 | 05:11.26       | 403.35                 | 0.47           | 5.21           | 0.133           | 0.061           | 02:13.90<br>02:13.71<br>-0.14 | 03:32.16<br>03:32.31<br>0.07  | 03:49.40<br>03:50.14<br>0.32  | 04:56.20<br>04:55.45<br>-0.25 | 07:35.20<br>07:36.88<br>0.37  | 13:13.00<br>13:08.12<br>-0.62 | 27:30.80<br>27:35.06<br>0.26  | 0.29      | 1:01:31.34                        | 2:08:33.60<br>2:09:58.26<br>1.10  |
| 1976 | 06:09.69       | 399.15                 | 0.43           | 5.12           | 0.119           | 0.061           | 02:13.90<br>02:14.19<br>0.21  | 03:32.16<br>03:31.46<br>-0.33 | 03:49.40<br>03:48.90<br>-0.22 | 04:51.52<br>04:52.51<br>0.34  | 07:35.20<br>07:36.88<br>0.37  | 13:13.00<br>13:08.12<br>-0.62 | 27:30.80<br>27:35.06<br>0.26  | 0.33      | 1:01:31.34                        | 2:08:33.60<br>2:09:58.26<br>1.10  |
| 1977 | 06:09.67       | 399.15                 | 0.43           | 5.14           | 0.119           | 0.061           | 02:13.90<br>02:14.19<br>0.21  | 03:32.16<br>03:31.46<br>-0.33 | 03:49.40<br>03:48.90<br>-0.22 | 04:51.52<br>04:52.51<br>0.34  | 07:35.20<br>07:36.86<br>0.37  | 13:12.87<br>13:08.03<br>-0.61 | 27:30.47<br>27:34.69<br>0.26  | 0.33      | 1:01:30.01                        | 2:08:33.60<br>2:09:54.33<br>1.05  |
| 1978 | 05:28.75       | 404.71                 | 0.43           | 5.03           | 0.117           | 0.062           | 02:13.90<br>02:14.19<br>0.21  | 03:32.16<br>03:31.46<br>-0.33 | 03:49.40<br>03:48.90<br>-0.22 | 04:51.52<br>04:52.51<br>0.34  | 07:32.10<br>07:33.82<br>0.38  | 13:08.40<br>13:03.39<br>-0.64 | 27:22.47<br>27:26.84<br>0.27  | 0.34      | 1:01:17.64                        | 2:08:33.60<br>2:09:39.60<br>0.86  |
| 1979 | 05:33.71       | 404.33                 | 0.42           | 5.02           | 0.117           | 0.062           | 02:13.90<br>02:14.13<br>0.17  | 03:32.03<br>03:31.33<br>-0.33 | 03:48.95<br>03:48.74<br>-0.09 | 04:51.52<br>04:52.26<br>0.25  | 07:32.10<br>07:33.82<br>0.38  | 13:08.40<br>13:03.39<br>-0.64 | 27:22.47<br>27:26.84<br>0.27  | 0.31      | 1:01:17.64                        | 2:08:33.60<br>2:09:39.60<br>0.86  |
| 1980 | 05:31.06       | 404.53                 | 0.44           | 5.02           | 0.121           | 0.062           | 02:13.40<br>02:13.59<br>0.15  | 03:31.36<br>03:30.93<br>-0.20 | 03:48.80<br>03:48.40<br>-0.18 | 04:51.52<br>04:52.21<br>0.24  | 07:32.10<br>07:33.82<br>0.38  | 13:08.40<br>13:03.39<br>-0.64 | 27:22.47<br>27:26.84<br>0.27  | 0.29      | 1:01:17.64                        | 2:08:33.60<br>2:09:39.60<br>0.86  |
| 1981 | 05:20.04       | 405.83                 | 0.47           | 5.02           | 0.132           | 0.062           | 02:12.18<br>02:12.44<br>0.20  | 03:31.36<br>03:30.11<br>-0.59 | 03:47.33<br>03:47.72<br>0.17  | 04:51.52<br>04:52.19<br>0.23  | 07:32.10<br>07:33.33<br>0.27  | 13:06.20<br>13:02.63<br>-0.45 | 27:22.47<br>27:25.56<br>0.19  | 0.30      | 1:01:15.61                        | 2:08:18.00<br>2:09:37.16<br>1.03  |
| 1982 | 05:06.79       | 408.09                 | 0.47           | 4.96           | 0.131           | 0.062           | 02:12.18<br>02:12.44<br>0.20  | 03:31.36<br>03:30.11<br>-0.59 | 03:47.33<br>03:47.72<br>0.17  | 04:51.52<br>04:52.19<br>0.23  | 07:32.10<br>07:32.02<br>-0.02 | 13:00.41<br>13:00.65<br>0.03  | 27:22.47<br>27:22.27<br>-0.01 | 0.18      | 1:01:10.63                        | 2:08:18.00<br>2:09:31.94<br>0.96  |
| 1983 | 05:09.75       | 407.84                 | 0.47           | 4.96           | 0.131           | 0.062           | 02:12.18<br>02:12.36<br>0.13  | 03:30.77<br>03:29.97<br>-0.38 | 03:47.33<br>03:47.56<br>0.10  | 04:51.52<br>04:51.97<br>0.15  | 07:32.10<br>07:32.02<br>-0.02 | 13:00.41<br>13:00.65<br>0.03  | 27:22.47<br>27:22.27<br>-0.01 | 0.12      | 1:01:10.63                        | 2:08:18.00<br>2:09:31.94<br>0.96  |
| 1984 | 05:19.08       | 406.26                 | 0.47           | 5.44           | 0.132           | 0.059           | 02:12.18<br>02:12.36<br>0.13  | 03:30.77<br>03:29.97<br>-0.38 | 03:47.33<br>03:47.56<br>0.10  | 04:51.52<br>04:51.97<br>0.15  | 07:32.10<br>07:32.39<br>0.06  | 13:00.41<br>12:59.56<br>-0.11 | 27:13.81<br>27:14.54<br>0.04  | 0.14      | 1:00:38.71                        | 2:08:05.00<br>2:07:51.95<br>-0.17 |
| 1985 | 05:33.38       | 405.21                 | 0.47           | 5.42           | 0.131           | 0.059           | 02:12.18<br>02:12.09<br>-0.07 | 03:29.46<br>03:29.38<br>-0.04 | 03:46.32<br>03:46.89<br>0.25  | 04:51.39<br>04:50.97<br>-0.14 | 07:32.10<br>07:32.39<br>0.06  | 13:00.40<br>12:59.56<br>-0.11 | 27:13.81<br>27:14.53<br>0.04  | 0.10      | 1:00:55.00<br>1:00:38.71<br>-0.45 | 2:07:12.00<br>2:07:51.94<br>0.52  |

| Year | t <sub>c</sub> | v <sub>m</sub> [m/min] | E <sub>s</sub> | E <sub>l</sub> | Y <sub>an</sub> | Y <sub>ae</sub> | 1000                          | 1500                          | 1609.34                      | 2000                          | 3000                          | 5000                          | 10 000                        | av.err[%] | Halfmarathon                      | Marathon                          |
|------|----------------|------------------------|----------------|----------------|-----------------|-----------------|-------------------------------|-------------------------------|------------------------------|-------------------------------|-------------------------------|-------------------------------|-------------------------------|-----------|-----------------------------------|-----------------------------------|
| 1986 | 05:33.38       | 405.21                 | 0.47           | 5.42           | 0.131           | 0.059           | 02:12.18<br>02:12.09<br>-0.07 | 03:29.46<br>03:29.38<br>-0.04 | 03:46.32<br>03:46.89<br>0.25 | 04:51.39<br>04:50.97<br>-0.14 | 07:32.10<br>07:32.39<br>0.06  | 13:00.40<br>12:59.56<br>-0.11 | 27:13.81<br>27:14.53<br>0.04  | 0.10      | 1:00:43.00<br>1:00:38.71<br>-0.12 | 2:07:12.00<br>2:07:51.94<br>0.52  |
| 1987 | 05:35.22       | 405.49                 | 0.46           | 5.38           | 0.129           | 0.059           | 02:12.18<br>02:12.15<br>-0.02 | 03:29.46<br>03:29.28<br>-0.09 | 03:46.32<br>03:46.73<br>0.18 | 04:50.81<br>04:50.60<br>-0.07 | 07:32.10<br>07:31.93<br>-0.04 | 12:58.39<br>12:58.87<br>0.06  | 27:13.81<br>27:13.40<br>-0.02 | 0.07      | 1:00:10.00<br>1:00:37.03<br>0.75  | 2:07:12.00<br>2:07:50.26<br>0.50  |
| 1988 | 05:35.22       | 405.49                 | 0.46           | 5.38           | 0.129           | 0.059           | 02:12.18<br>02:12.15<br>-0.02 | 03:29.46<br>03:29.28<br>-0.09 | 03:46.32<br>03:46.73<br>0.18 | 04:50.81<br>04:50.60<br>-0.07 | 07:32.10<br>07:31.93<br>-0.04 | 12:58.39<br>12:58.87<br>0.06  | 27:13.81<br>27:13.40<br>-0.02 | 0.07      | 1:00:10.00<br>1:00:37.03<br>0.75  | 2:06:50.00<br>2:07:50.26<br>0.79  |
| 1989 | 05:15.55       | 408.64                 | 0.46           | 5.24           | 0.128           | 0.060           | 02:12.18<br>02:12.15<br>-0.02 | 03:29.46<br>03:29.28<br>-0.09 | 03:46.32<br>03:46.73<br>0.18 | 04:50.81<br>04:50.60<br>-0.07 | 07:29.45<br>07:30.15<br>0.16  | 12:58.39<br>12:56.37<br>-0.26 | 27:08.23<br>27:09.97<br>0.11  | 0.13      | 1:00:10.00<br>1:00:34.25<br>0.67  | 2:06:50.00<br>2:07:55.15<br>0.86  |
| 1990 | 05:15.55       | 408.64                 | 0.46           | 5.24           | 0.128           | 0.060           | 02:12.18<br>02:12.15<br>-0.02 | 03:29.46<br>03:29.28<br>-0.09 | 03:46.32<br>03:46.73<br>0.18 | 04:50.81<br>04:50.60<br>-0.07 | 07:29.45<br>07:30.15<br>0.16  | 12:58.39<br>12:56.37<br>-0.26 | 27:08.23<br>27:09.97<br>0.11  | 0.13      | 1:00:10.00<br>1:00:34.25<br>0.67  | 2:06:50.00<br>2:07:55.15<br>0.86  |
| 1991 | 05:15.55       | 408.64                 | 0.46           | 5.24           | 0.128           | 0.060           | 02:12.18<br>02:12.15<br>-0.02 | 03:29.46<br>03:29.28<br>-0.09 | 03:46.32<br>03:46.73<br>0.18 | 04:50.81<br>04:50.60<br>-0.07 | 07:29.45<br>07:30.15<br>0.16  | 12:58.39<br>12:56.37<br>-0.26 | 27:08.23<br>27:09.97<br>0.11  | 0.13      | 1:00:10.00<br>1:00:34.25<br>0.67  | 2:06:50.00<br>2:07:55.15<br>0.86  |
| 1992 | 05:13.75       | 409.20                 | 0.46           | 5.15           | 0.128           | 0.061           | 02:12.18<br>02:12.06<br>-0.09 | 03:28.86<br>03:29.13<br>0.13  | 03:46.32<br>03:46.57<br>0.11 | 04:50.81<br>04:50.39<br>-0.14 | 07:28.96<br>07:29.77<br>0.18  | 12:58.39<br>12:56.04<br>-0.30 | 27:08.23<br>27:10.26<br>0.12  | 0.15      | 1:00:10.00<br>1:00:37.55<br>0.76  | 2:06:50.00<br>2:08:08.04<br>1.03  |
| 1993 | 05:37.45       | 406.53                 | 0.45           | 5.75           | 0.127           | 0.057           | 02:12.18<br>02:11.90<br>-0.22 | 03:28.86<br>03:28.68<br>-0.09 | 03:44.39<br>03:46.05<br>0.74 | 04:50.81<br>04:49.57<br>-0.43 | 07:28.96<br>07:30.20<br>0.28  | 12:58.39<br>12:54.79<br>-0.46 | 26:58.38<br>27:01.50<br>0.19  | 0.34      | 59:47.00<br>1:00:01.55<br>0.41    | 2:06:50.00<br>2:06:15.78<br>-0.45 |
| 1994 | 04:58.11       | 412.91                 | 0.45           | 5.13           | 0.125           | 0.061           | 02:12.18<br>02:11.90<br>-0.22 | 03:28.86<br>03:28.68<br>-0.09 | 03:44.39<br>03:46.05<br>0.74 | 04:50.81<br>04:49.57<br>-0.43 | 07:25.11<br>07:27.01<br>0.43  | 12:56.96<br>12:51.43<br>-0.71 | 26:56.23<br>27:01.07<br>0.30  | 0.42      | 59:47.00<br>1:00:18.38<br>0.87    | 2:06:50.00<br>2:07:30.47<br>0.53  |
| 1995 | 05:22.76       | 412.34                 | 0.42           | 5.71           | 0.115           | 0.057           | 02:12.18<br>02:11.98<br>-0.15 | 03:27.37<br>03:27.77<br>0.19  | 03:44.39<br>03:44.86<br>0.21 | 04:47.88<br>04:47.18<br>-0.24 | 07:25.11<br>07:24.72<br>-0.09 | 12:44.39<br>12:45.52<br>0.15  | 26:43.53<br>26:42.58<br>-0.06 | 0.16      | 59:47.00<br>59:20.82<br>-0.73     | 2:06:50.00<br>2:04:52.91<br>-1.54 |
| 1996 | 04:47.88       | 417.98                 | 0.41           | 5.32           | 0.112           | 0.060           | 02:12.18<br>02:12.01<br>-0.13 | 03:27.37<br>03:27.72<br>0.17  | 03:44.39<br>03:44.78<br>0.17 | 04:47.88<br>04:47.00<br>-0.31 | 07:20.67<br>07:21.98<br>0.30  | 12:44.39<br>12:42.13<br>-0.30 | 26:38.08<br>26:39.59<br>0.09  | 0.21      | 59:47.00<br>59:25.19<br>-0.61     | 2:06:50.00<br>2:05:26.40<br>-1.10 |
| 1997 | 04:47.88       | 417.93                 | 0.41           | 5.93           | 0.112           | 0.056           | 02:12.18<br>02:12.00<br>-0.14 | 03:27.37<br>03:27.73<br>0.17  | 03:44.39<br>03:44.80<br>0.18 | 04:47.88<br>04:47.04<br>-0.29 | 07:20.67<br>07:21.28<br>0.14  | 12:39.74<br>12:39.18<br>-0.07 | 26:27.85<br>26:27.98<br>0.01  | 0.14      | 59:47.00<br>58:44.87<br>-1.73     | 2:06:50.00<br>2:03:29.61<br>-2.63 |
| 1998 | 04:53.78       | 417.38                 | 0.41           | 6.20           | 0.114           | 0.055           | 02:12.18<br>02:11.76<br>-0.32 | 03:26.00<br>03:27.43<br>0.70  | 03:44.39<br>03:44.49<br>0.04 | 04:47.88<br>04:46.71<br>-0.41 | 07:20.67<br>07:21.08<br>0.09  | 12:39.36<br>12:38.16<br>-0.16 | 26:22.75<br>26:23.78<br>0.06  | 0.25      | 59:17.00<br>58:30.05<br>-1.32     | 2:06:05.00<br>2:02:46.52<br>-2.62 |
| 1999 | 05:45.46       | 413.68                 | 0.38           | 6.10           | 0.104           | 0.055           | 02:11.96<br>02:11.80<br>-0.12 | 03:26.00<br>03:26.48<br>0.23  | 03:43.13<br>03:43.26<br>0.06 | 04:44.79<br>04:44.31<br>-0.17 | 07:20.67<br>07:21.08<br>0.09  | 12:39.36<br>12:38.16<br>-0.16 | 26:22.75<br>26:23.78<br>0.06  | 0.13      | 59:17.00<br>58:30.05<br>-1.32     | 2:05:42.00<br>2:02:46.52<br>-2.33 |
| 2000 | 05:45.46       | 413.68                 | 0.38           | 6.10           | 0.104           | 0.055           | 02:11.96<br>02:11.80<br>-0.12 | 03:26.00<br>03:26.48<br>0.23  | 03:43.13<br>03:43.26<br>0.06 | 04:44.79<br>04:44.31<br>-0.17 | 07:20.67<br>07:21.08<br>0.09  | 12:39.36<br>12:38.16<br>-0.16 | 26:22.75<br>26:23.78<br>0.06  | 0.13      | 59:06.00<br>58:30.05<br>-1.01     | 2:05:42.00<br>2:02:46.52<br>-2.33 |
| 2001 | 05:45.46       | 413.68                 | 0.38           | 6.10           | 0.104           | 0.055           | 02:11.96<br>02:11.80<br>-0.12 | 03:26.00<br>03:26.48<br>0.23  | 03:43.13<br>03:43.26<br>0.06 | 04:44.79<br>04:44.31<br>-0.17 | 07:20.67<br>07:21.08<br>0.09  | 12:39.36<br>12:38.16<br>-0.16 | 26:22.75<br>26:23.78<br>0.06  | 0.13      | 59:06.00<br>58:30.05<br>-1.01     | 2:05:42.00<br>2:02:46.52<br>-2.33 |
| 2002 | 05:45.46       | 413.68                 | 0.38           | 6.10           | 0.104           | 0.055           | 02:11.96<br>02:11.80<br>-0.12 | 03:26.00<br>03:26.48<br>0.23  | 03:43.13<br>03:43.26<br>0.06 | 04:44.79<br>04:44.31<br>-0.17 | 07:20.67<br>07:21.08<br>0.09  | 12:39.36<br>12:38.16<br>-0.16 | 26:22.75<br>26:23.78<br>0.06  | 0.13      | 59:06.00<br>58:30.05<br>-1.01     | 2:05:37.80<br>2:02:46.52<br>-2.27 |

| Year | t <sub>c</sub> | v <sub>m</sub> [m/min] | E <sub>s</sub> | E <sub>l</sub> | Y <sub>an</sub> | Y <sub>ae</sub> | 1000     | 1500     | 1609.34  | 2000     | 3000     | 5000     | 10 000   | av.err[%] | Halfmarathon | Marathon   |
|------|----------------|------------------------|----------------|----------------|-----------------|-----------------|----------|----------|----------|----------|----------|----------|----------|-----------|--------------|------------|
| 2003 | 05:45.46       | 413.68                 | 0.38           | 6.10           | 0.104           | 0.055           | 02:11.96 | 03:26.00 | 03:43.13 | 04:44.79 | 07:20.67 | 12:39.36 | 26:22.75 | 0.13      | 59:06.00     | 2:04:55.00 |
|      |                |                        |                |                |                 |                 | 02:11.80 | 03:26.48 | 03:43.26 | 04:44.31 | 07:21.08 | 12:38.16 | 26:23.78 |           | 58:30.05     | 2:02:46.52 |
|      |                |                        |                |                |                 |                 | -0.12    | 0.23     | 0.06     | -0.17    | 0.09     | -0.16    | 0.06     |           | -1.01        | -1.71      |
| 2004 | 05:41.77       | 414.14                 | 0.38           | 6.28           | 0.104           | 0.054           | 02:11.96 | 03:26.00 | 03:43.13 | 04:44.79 | 07:20.67 | 12:37.35 | 26:20.31 | 0.09      | 59:06.00     | 2:04:55.00 |
|      |                |                        |                |                |                 |                 | 02:11.80 | 03:26.48 | 03:43.26 | 04:44.31 | 07:20.73 | 12:37.16 | 26:20.47 |           | 58:19.50     | 2:02:17.40 |
|      |                |                        |                |                |                 |                 | -0.12    | 0.23     | 0.06     | -0.17    | 0.01     | -0.02    | 0.01     |           | -1.31        | -2.10      |
| 2005 | 05:45.68       | 413.65                 | 0.38           | 6.55           | 0.104           | 0.053           | 02:11.96 | 03:26.00 | 03:43.13 | 04:44.79 | 07:20.67 | 12:37.35 | 26:17.53 | 0.10      | 59:05.00     | 2:04:55.00 |
|      |                |                        |                |                |                 |                 | 02:11.80 | 03:26.48 | 03:43.26 | 04:44.31 | 07:20.86 | 12:36.81 | 26:17.99 |           | 58:09.46     | 2:01:46.52 |
|      |                |                        |                |                |                 |                 | -0.12    | 0.23     | 0.06     | -0.17    | 0.04     | -0.07    | 0.03     |           | -1.57        | -2.51      |
| 2006 | 05:45.68       | 413.65                 | 0.38           | 6.55           | 0.104           | 0.053           | 02:11.96 | 03:26.00 | 03:43.13 | 04:44.79 | 07:20.67 | 12:37.35 | 26:17.53 | 0.10      | 58:55.00     | 2:04:55.00 |
|      |                |                        |                |                |                 |                 | 02:11.80 | 03:26.48 | 03:43.26 | 04:44.31 | 07:20.86 | 12:36.81 | 26:17.99 |           | 58:09.46     | 2:01:46.52 |
|      |                |                        |                |                |                 |                 | -0.12    | 0.23     | 0.06     | -0.17    | 0.04     | -0.07    | 0.03     |           | -1.29        | -2.51      |
| 2007 | 05:45.68       | 413.65                 | 0.38           | 6.55           | 0.104           | 0.053           | 02:11.96 | 03:26.00 | 03:43.13 | 04:44.79 | 07:20.67 | 12:37.35 | 26:17.53 | 0.10      | 58:33.00     | 2:04:26.00 |
|      |                |                        |                |                |                 |                 | 02:11.80 | 03:26.48 | 03:43.26 | 04:44.31 | 07:20.86 | 12:36.81 | 26:17.99 |           | 58:09.46     | 2:01:46.52 |
|      |                |                        |                |                |                 |                 | -0.12    | 0.23     | 0.06     | -0.17    | 0.04     | -0.07    | 0.03     |           | -0.67        | -2.14      |
| 2008 | 05:45.68       | 413.65                 | 0.38           | 6.55           | 0.104           | 0.053           | 02:11.96 | 03:26.00 | 03:43.13 | 04:44.79 | 07:20.67 | 12:37.35 | 26:17.53 | 0.10      | 58:33.00     | 2:03:58.20 |
|      |                |                        |                |                |                 |                 | 02:11.80 | 03:26.48 | 03:43.26 | 04:44.31 | 07:20.86 | 12:36.81 | 26:17.99 |           | 58:09.46     | 2:01:46.52 |
|      |                |                        |                |                |                 |                 | -0.12    | 0.23     | 0.06     | -0.17    | 0.04     | -0.07    | 0.03     |           | -0.67        | -1.77      |
| 2009 | 05:45.68       | 413.65                 | 0.38           | 6.55           | 0.104           | 0.053           | 02:11.96 | 03:26.00 | 03:43.13 | 04:44.79 | 07:20.67 | 12:37.35 | 26:17.53 | 0.10      | 58:33.00     | 2:03:58.20 |
|      |                |                        |                |                |                 |                 | 02:11.80 | 03:26.48 | 03:43.26 | 04:44.31 | 07:20.86 | 12:36.81 | 26:17.99 |           | 58:09.46     | 2:01:46.52 |
|      |                |                        |                |                |                 |                 | -0.12    | 0.23     | 0.06     | -0.17    | 0.04     | -0.07    | 0.03     |           | -0.67        | -1.77      |
| 2010 | 05:45.68       | 413.65                 | 0.38           | 6.55           | 0.104           | 0.053           | 02:11.96 | 03:26.00 | 03:43.13 | 04:44.79 | 07:20.67 | 12:37.35 | 26:17.53 | 0.10      | 58:23.00     | 2:03:58.20 |
|      |                |                        |                |                |                 |                 | 02:11.80 | 03:26.48 | 03:43.26 | 04:44.31 | 07:20.86 | 12:36.81 | 26:17.99 |           | 58:09.46     | 2:01:46.52 |
|      |                |                        |                |                |                 |                 | -0.12    | 0.23     | 0.06     | -0.17    | 0.04     | -0.07    | 0.03     |           | -0.39        | -1.77      |
| 2011 | 05:45.68       | 413.65                 | 0.38           | 6.55           | 0.104           | 0.053           | 02:11.96 | 03:26.00 | 03:43.13 | 04:44.79 | 07:20.67 | 12:37.35 | 26:17.53 | 0.10      | 58:23.00     | 2:03:38.00 |
|      |                |                        |                |                |                 |                 | 02:11.80 | 03:26.48 | 03:43.26 | 04:44.31 | 07:20.86 | 12:36.81 | 26:17.99 |           | 58:09.46     | 2:01:46.52 |
|      |                |                        |                |                |                 |                 | -0.12    | 0.23     | 0.06     | -0.17    | 0.04     | -0.07    | 0.03     |           | -0.39        | -1.50      |
| 2012 | 05:45.68       | 413.65                 | 0.38           | 6.55           | 0.104           | 0.053           | 02:11.96 | 03:26.00 | 03:43.13 | 04:44.79 | 07:20.67 | 12:37.35 | 26:17.53 | 0.10      | 58:23.00     | 2:03:38.00 |
|      |                |                        |                |                |                 |                 | 02:11.80 | 03:26.48 | 03:43.26 | 04:44.31 | 07:20.86 | 12:36.81 | 26:17.99 |           | 58:09.46     | 2:01:46.52 |
|      |                |                        |                |                |                 |                 | -0.12    | 0.23     | 0.06     | -0.17    | 0.04     | -0.07    | 0.03     |           | -0.39        | -1.50      |
| 2013 | 05:45.68       | 413.65                 | 0.38           | 6.55           | 0.104           | 0.053           | 02:11.96 | 03:26.00 | 03:43.13 | 04:44.79 | 07:20.67 | 12:37.35 | 26:17.53 | 0.10      | 58:23.00     | 2:03:22.20 |
|      |                |                        |                |                |                 |                 | 02:11.80 | 03:26.48 | 03:43.26 | 04:44.31 | 07:20.86 | 12:36.81 | 26:17.99 |           | 58:09.46     | 2:01:46.52 |
|      |                |                        |                |                |                 |                 | -0.12    | 0.23     | 0.06     | -0.17    | 0.04     | -0.07    | 0.03     |           | -0.39        | -1.29      |
| 2014 | 05:45.68       | 413.65                 | 0.38           | 6.55           | 0.104           | 0.053           | 02:11.96 | 03:26.00 | 03:43.13 | 04:44.79 | 07:20.67 | 12:37.35 | 26:17.53 | 0.10      | 58:23.00     | 2:02:56.40 |
|      |                |                        |                |                |                 |                 | 02:11.80 | 03:26.48 | 03:43.26 | 04:44.31 | 07:20.86 | 12:36.81 | 26:17.99 |           | 58:09.46     | 2:01:46.52 |
|      |                |                        |                |                |                 |                 | -0.12    | 0.23     | 0.06     | -0.17    | 0.04     | -0.07    | 0.03     |           | -0.39        | -0.95      |
| 2015 | 05:45.68       | 413.65                 | 0.38           | 6.55           | 0.104           | 0.053           | 02:11.96 | 03:26.00 | 03:43.13 | 04:44.79 | 07:20.67 | 12:37.35 | 26:17.53 | 0.10      | 58:23.00     | 2:02:56.40 |
|      |                |                        |                |                |                 |                 | 02:11.80 | 03:26.48 | 03:43.26 | 04:44.31 | 07:20.86 | 12:36.81 | 26:17.99 |           | 58:09.46     | 2:01:46.52 |
|      |                |                        |                |                |                 |                 | -0.12    | 0.23     | 0.06     | -0.17    | 0.04     | -0.07    | 0.03     |           | -0.39        | -0.95      |
| 2016 | 05:45.68       | 413.65                 | 0.38           | 6.55           | 0.104           | 0.053           | 02:11.96 | 03:26.00 | 03:43.13 | 04:44.79 | 07:20.67 | 12:37.35 | 26:17.53 | 0.10      | 58:23.00     | 2:02:56.40 |
|      |                |                        |                |                |                 |                 | 02:11.80 | 03:26.48 | 03:43.26 | 04:44.31 | 07:20.86 | 12:36.81 | 26:17.99 |           | 58:09.46     | 2:01:46.52 |
|      |                |                        |                |                |                 |                 | -0.12    | 0.23     | 0.06     | -0.17    | 0.04     | -0.07    | 0.03     |           | -0.39        | -0.95      |
| 2017 | 05:45.68       | 413.65                 | 0.38           | 6.55           | 0.104           | 0.053           | 02:11.96 | 03:26.00 | 03:43.13 | 04:44.79 | 07:20.67 | 12:37.35 | 26:17.53 | 0.10      | 58:23.00     | 2:02:56.40 |
|      |                |                        |                |                |                 |                 | 02:11.80 | 03:26.48 | 03:43.26 | 04:44.31 | 07:20.86 | 12:36.81 | 26:17.99 |           | 58:09.46     | 2:01:46.52 |
|      |                |                        |                |                |                 |                 | -0.12    | 0.23     | 0.06     | -0.17    | 0.04     | -0.07    | 0.03     |           | -0.39        | -0.95      |
| 2018 | 05:45.68       | 413.65                 | 0.38           | 6.55           | 0.104           | 0.053           | 02:11.96 | 03:26.00 | 03:43.13 | 04:44.79 | 07:20.67 | 12:37.35 | 26:17.53 | 0.10      | 58:18.00     | 2:01:39.00 |
|      |                |                        |                |                |                 |                 | 02:11.80 | 03:26.48 | 03:43.26 | 04:44.31 | 07:20.86 | 12:36.81 | 26:17.99 |           | 58:09.46     | 2:01:46.52 |
|      |                |                        |                |                |                 |                 | -0.12    | 0.23     | 0.06     | -0.17    | 0.04     | -0.07    | 0.03     |           | -0.24        | 0.10       |
| 2019 | 05:45.68       | 413.65                 | 0.38           | 6.55           | 0.104           | 0.053           | 02:11.96 | 03:26.00 | 03:43.13 | 04:44.79 | 07:20.67 | 12:37.35 | 26:17.53 | 0.10      | 58:01.00     | 2:01:39.00 |
|      |                |                        |                |                |                 |                 | 02:11.80 | 03:26.48 | 03:43.26 | 04:44.31 | 07:20.86 | 12:36.81 | 26:17.99 |           | 58:09.46     | 2:01:46.52 |
|      |                |                        |                |                |                 |                 | -0.12    | 0.23     | 0.06     | -0.17    | 0.04     | -0.07    | 0.03     |           | 0.24         | 0.10       |

| Year | t <sub>c</sub> | v <sub>m</sub> [m/min] | E <sub>s</sub> | E <sub>l</sub> | γ <sub>an</sub> | γ <sub>ae</sub> | 1000     | 1500     | 1609.34  | 2000     | 3000     | 5000     | 10 000   | av. err [%] | Halfmarathon | Marathon   |
|------|----------------|------------------------|----------------|----------------|-----------------|-----------------|----------|----------|----------|----------|----------|----------|----------|-------------|--------------|------------|
| 2020 | 05:47.74       | 413.39                 | 0.38           | 7.24           | 0.104           | 0.051           | 02:11.96 | 03:26.00 | 03:43.13 | 04:44.79 | 07:20.67 | 12:35.36 | 26:11.00 | 0.09        | 57:32.00     | 2:01:39.00 |
|      |                |                        |                |                |                 |                 | 02:11.80 | 03:26.48 | 03:43.26 | 04:44.31 | 07:20.69 | 12:35.29 | 26:11.06 |             | 57:44.30     | 2:00:32.80 |
|      |                |                        |                |                |                 |                 | -0.12    | 0.23     | 0.06     | -0.17    | 0.01     | -0.01    | 0.00     |             | 0.36         | -0.91      |
| 2021 | 05:47.74       | 413.39                 | 0.38           | 7.24           | 0.104           | 0.051           | 02:11.96 | 03:26.00 | 03:43.13 | 04:44.79 | 07:20.67 | 12:35.36 | 26:11.00 | 0.09        | 57:31.00     | 2:01:39.00 |
|      |                |                        |                |                |                 |                 | 02:11.80 | 03:26.48 | 03:43.26 | 04:44.31 | 07:20.69 | 12:35.29 | 26:11.06 |             | 57:44.30     | 2:00:32.80 |
|      |                |                        |                |                |                 |                 | -0.12    | 0.23     | 0.06     | -0.17    | 0.01     | -0.01    | 0.00     |             | 0.39         | -0.91      |
| 2022 | 05:47.74       | 413.39                 | 0.38           | 7.24           | 0.104           | 0.051           | 02:11.96 | 03:26.00 | 03:43.13 | 04:44.79 | 07:20.67 | 12:35.36 | 26:11.00 | 0.09        | 57:31.00     | 2:01:09.00 |
|      |                |                        |                |                |                 |                 | 02:11.80 | 03:26.48 | 03:43.26 | 04:44.31 | 07:20.69 | 12:35.29 | 26:11.06 |             | 57:44.30     | 2:00:32.80 |
|      |                |                        |                |                |                 |                 | -0.12    | 0.23     | 0.06     | -0.17    | 0.01     | -0.01    | 0.00     |             | 0.39         | -0.50      |
| 2023 | 06:23.09       | 411.37                 | 0.36           | 7.17           | 0.099           | 0.051           | 02:11.96 | 03:26.00 | 03:43.13 | 04:43.13 | 07:20.67 | 12:35.36 | 26:11.00 | 0.04        | 57:31.00     | 2:00:35.00 |
|      |                |                        |                |                |                 |                 | 02:11.97 | 03:26.17 | 03:42.81 | 04:43.27 | 07:20.69 | 12:35.29 | 26:11.06 |             | 57:44.30     | 2:00:32.80 |
|      |                |                        |                |                |                 |                 | 0.01     | 0.08     | -0.14    | 0.05     | 0.01     | -0.01    | 0.00     |             | 0.39         | -0.03      |

# World Records Women

| Year | t <sub>c</sub> | v <sub>m</sub> [m/min] | E <sub>s</sub> | E <sub>l</sub> | Y <sub>an</sub> | Y <sub>ae</sub> | 1000                          | 1500                         | 1609.34                       | 2000                          | 3000                         | 5000                          | 10 000                       | av.err[%] | Halfmarathon                      | Marathon                          |
|------|----------------|------------------------|----------------|----------------|-----------------|-----------------|-------------------------------|------------------------------|-------------------------------|-------------------------------|------------------------------|-------------------------------|------------------------------|-----------|-----------------------------------|-----------------------------------|
| 1984 | 07:40.08       | 356.87                 | 0.34           | 3.90           | 0.093           | 0.073           | 02:33.80<br>02:32.46<br>-0.87 | 03:52.47<br>03:57.58<br>2.20 | 04:17.44<br>04:16.63<br>-0.31 | 05:28.72<br>05:25.79<br>-0.89 | 08:22.62<br>08:28.08<br>1.09 | 14:58.89<br>14:42.89<br>-1.78 | 31:00.00<br>31:14.64<br>0.79 | 1.13      | 1:08:34.00<br>1:10:38.07<br>3.02  | 2:22:43.00<br>2:31:23.71<br>6.08  |
| 1985 | 06:25.29       | 363.14                 | 0.33           | 3.93           | 0.091           | 0.073           | 02:33.80<br>02:32.40<br>-0.91 | 03:52.47<br>03:57.41<br>2.12 | 04:16.71<br>04:16.43<br>-0.11 | 05:28.72<br>05:25.47<br>-0.99 | 08:22.62<br>08:25.71<br>0.62 | 14:48.07<br>14:39.06<br>-1.02 | 30:59.42<br>31:07.42<br>0.43 | 0.88      | 1:08:34.00<br>1:10:24.32<br>2.68  | 2:21:06.00<br>2:31:00.30<br>7.02  |
| 1986 | 07:07.94       | 359.72                 | 0.34           | 5.63           | 0.091           | 0.058           | 02:33.80<br>02:32.41<br>-0.91 | 03:52.47<br>03:57.40<br>2.12 | 04:16.71<br>04:16.42<br>-0.11 | 05:28.69<br>05:25.45<br>-0.99 | 08:22.62<br>08:25.25<br>0.52 | 14:37.33<br>14:29.67<br>-0.87 | 30:13.74<br>30:20.49<br>0.37 | 0.84      | 1:08:34.00<br>1:07:24.67<br>-1.69 | 2:21:06.00<br>2:21:50.32<br>0.52  |
| 1987 | 07:07.94       | 359.72                 | 0.34           | 5.63           | 0.091           | 0.058           | 02:33.80<br>02:32.41<br>-0.91 | 03:52.47<br>03:57.40<br>2.12 | 04:16.71<br>04:16.42<br>-0.11 | 05:28.69<br>05:25.45<br>-0.99 | 08:22.62<br>08:25.25<br>0.52 | 14:37.33<br>14:29.67<br>-0.87 | 30:13.74<br>30:20.49<br>0.37 | 0.84      | 1:06:40.00<br>1:07:24.67<br>1.12  | 2:21:06.00<br>2:21:50.32<br>0.52  |
| 1988 | 07:07.94       | 359.72                 | 0.34           | 5.63           | 0.091           | 0.058           | 02:33.80<br>02:32.41<br>-0.91 | 03:52.47<br>03:57.40<br>2.12 | 04:16.71<br>04:16.42<br>-0.11 | 05:28.69<br>05:25.45<br>-0.99 | 08:22.62<br>08:25.25<br>0.52 | 14:37.33<br>14:29.67<br>-0.87 | 30:13.74<br>30:20.49<br>0.37 | 0.84      | 1:06:40.00<br>1:07:24.67<br>1.12  | 2:21:06.00<br>2:21:50.32<br>0.52  |
| 1989 | 07:30.41       | 358.65                 | 0.33           | 5.60           | 0.091           | 0.058           | 02:33.80<br>02:32.32<br>-0.96 | 03:52.47<br>03:57.15<br>2.01 | 04:15.61<br>04:16.12<br>0.20  | 05:28.69<br>05:24.97<br>-1.13 | 08:22.62<br>08:25.25<br>0.52 | 14:37.33<br>14:29.67<br>-0.87 | 30:13.74<br>30:20.49<br>0.37 | 0.87      | 1:06:40.00<br>1:07:24.67<br>1.12  | 2:21:06.00<br>2:21:50.32<br>0.52  |
| 1990 | 06:03.72       | 363.10                 | 0.42           | 5.72           | 0.117           | 0.057           | 02:30.67<br>02:29.72<br>-0.63 | 03:52.47<br>03:55.93<br>1.49 | 04:15.61<br>04:15.38<br>-0.09 | 05:28.69<br>05:26.35<br>-0.71 | 08:22.62<br>08:25.25<br>0.52 | 14:37.33<br>14:29.67<br>-0.87 | 30:13.74<br>30:20.49<br>0.37 | 0.67      | 1:06:40.00<br>1:07:24.67<br>1.12  | 2:21:06.00<br>2:21:50.32<br>0.52  |
| 1991 | 06:03.72       | 363.10                 | 0.42           | 5.72           | 0.117           | 0.057           | 02:30.67<br>02:29.72<br>-0.63 | 03:52.47<br>03:55.93<br>1.49 | 04:15.61<br>04:15.38<br>-0.09 | 05:28.69<br>05:26.35<br>-0.71 | 08:22.62<br>08:25.25<br>0.52 | 14:37.33<br>14:29.67<br>-0.87 | 30:13.74<br>30:20.49<br>0.37 | 0.67      | 1:06:40.00<br>1:07:24.67<br>1.12  | 2:21:06.00<br>2:21:50.32<br>0.52  |
| 1992 | 06:03.72       | 363.10                 | 0.42           | 5.72           | 0.117           | 0.057           | 02:30.67<br>02:29.72<br>-0.63 | 03:52.47<br>03:55.93<br>1.49 | 04:15.61<br>04:15.38<br>-0.09 | 05:28.69<br>05:26.35<br>-0.71 | 08:22.62<br>08:25.25<br>0.52 | 14:37.33<br>14:29.67<br>-0.87 | 30:13.74<br>30:20.49<br>0.37 | 0.67      | 1:06:40.00<br>1:07:24.67<br>1.12  | 2:21:06.00<br>2:21:50.32<br>0.52  |
| 1993 | 05:28.69       | 369.65                 | 0.40           | 6.28           | 0.108           | 0.054           | 02:30.67<br>02:29.63<br>-0.69 | 03:50.46<br>03:54.97<br>1.96 | 04:15.61<br>04:14.18<br>-0.56 | 05:28.69<br>05:24.14<br>-1.38 | 08:06.11<br>08:18.22<br>2.49 | 14:37.33<br>14:16.20<br>-2.41 | 29:31.78<br>29:48.01<br>0.92 | 1.49      | 1:06:40.00<br>1:06:01.22<br>-0.97 | 2:21:06.00<br>2:18:30.19<br>-1.84 |
| 1994 | 05:25.36       | 371.56                 | 0.37           | 5.67           | 0.100           | 0.058           | 02:30.67<br>02:29.88<br>-0.53 | 03:50.46<br>03:54.55<br>1.78 | 04:15.61<br>04:13.56<br>-0.80 | 05:25.36<br>05:22.70<br>-0.82 | 08:06.11<br>08:16.54<br>2.15 | 14:37.33<br>14:15.00<br>-2.55 | 29:31.78<br>29:50.75<br>1.07 | 1.38      | 1:06:40.00<br>1:06:21.24<br>-0.47 | 2:21:06.00<br>2:19:42.63<br>-0.98 |
| 1995 | 05:25.36       | 371.14                 | 0.40           | 5.85           | 0.111           | 0.057           | 02:29.34<br>02:28.80<br>-0.36 | 03:50.46<br>03:53.97<br>1.52 | 04:15.61<br>04:13.15<br>-0.96 | 05:25.36<br>05:23.08<br>-0.70 | 08:06.11<br>08:16.90<br>2.22 | 14:36.45<br>14:15.08<br>-2.44 | 29:31.78<br>29:49.23<br>0.99 | 1.31      | 1:06:40.00<br>1:06:13.37<br>-0.67 | 2:21:06.00<br>2:19:16.26<br>-1.30 |
| 1996 | 05:25.36       | 372.02                 | 0.41           | 5.57           | 0.112           | 0.058           | 02:28.98<br>02:28.22<br>-0.51 | 03:50.46<br>03:53.22<br>1.20 | 04:12.56<br>04:12.37<br>-0.07 | 05:25.36<br>05:22.22<br>-0.97 | 08:06.11<br>08:16.03<br>2.04 | 14:36.45<br>14:14.46<br>-2.51 | 29:31.78<br>29:50.68<br>1.07 | 1.19      | 1:06:40.00<br>1:06:23.88<br>-0.40 | 2:21:06.00<br>2:19:54.34<br>-0.85 |
| 1997 | 05:25.36       | 372.42                 | 0.40           | 5.81           | 0.110           | 0.057           | 02:28.98<br>02:28.29<br>-0.47 | 03:50.46<br>03:53.11<br>1.15 | 04:12.56<br>04:12.21<br>-0.14 | 05:25.36<br>05:21.83<br>-1.08 | 08:06.11<br>08:15.15<br>1.86 | 14:28.09<br>14:12.19<br>-1.83 | 29:31.78<br>29:43.61<br>0.67 | 1.03      | 1:06:40.00<br>1:06:01.99<br>-0.95 | 2:21:06.00<br>2:18:54.73<br>-1.55 |
| 1998 | 05:25.36       | 372.42                 | 0.40           | 5.81           | 0.110           | 0.057           | 02:28.98<br>02:28.29<br>-0.47 | 03:50.46<br>03:53.11<br>1.15 | 04:12.56<br>04:12.21<br>-0.14 | 05:25.36<br>05:21.83<br>-1.08 | 08:06.11<br>08:15.15<br>1.86 | 14:28.09<br>14:12.19<br>-1.83 | 29:31.78<br>29:43.61<br>0.67 | 1.03      | 1:06:40.00<br>1:06:01.99<br>-0.95 | 2:20:47.00<br>2:18:54.73<br>-1.33 |
| 1999 | 05:25.36       | 372.42                 | 0.40           | 5.81           | 0.110           | 0.057           | 02:28.98<br>02:28.29<br>-0.47 | 03:50.46<br>03:53.11<br>1.15 | 04:12.56<br>04:12.21<br>-0.14 | 05:25.36<br>05:21.83<br>-1.08 | 08:06.11<br>08:15.15<br>1.86 | 14:28.09<br>14:12.19<br>-1.83 | 29:31.78<br>29:43.61<br>0.67 | 1.03      | 1:06:40.00<br>1:06:01.99<br>-0.95 | 2:20:43.00<br>2:18:54.73<br>-1.28 |
| 2000 | 05:25.36       | 372.42                 | 0.40           | 5.81           | 0.110           | 0.057           | 02:28.98<br>02:28.29<br>-0.47 | 03:50.46<br>03:53.11<br>1.15 | 04:12.56<br>04:12.21<br>-0.14 | 05:25.36<br>05:21.83<br>-1.08 | 08:06.11<br>08:15.15<br>1.86 | 14:28.09<br>14:12.19<br>-1.83 | 29:31.78<br>29:43.61<br>0.67 | 1.03      | 1:06:40.00<br>1:06:01.99<br>-0.95 | 2:20:43.00<br>2:18:54.73<br>-1.28 |

| Year | t <sub>c</sub> | v <sub>m</sub> [m/min] | E <sub>s</sub> | E <sub>l</sub> | Y <sub>an</sub> | Y <sub>ae</sub> | 1000                          | 1500                         | 1609.34                       | 2000                          | 3000                         | 5000                          | 10 000                        | av.err[%] | Halfmarathon                      | Marathon                          |
|------|----------------|------------------------|----------------|----------------|-----------------|-----------------|-------------------------------|------------------------------|-------------------------------|-------------------------------|------------------------------|-------------------------------|-------------------------------|-----------|-----------------------------------|-----------------------------------|
| 2001 | 05:25.36       | 372.42                 | 0.40           | 5.81           | 0.110           | 0.057           | 02:28.98<br>02:28.29<br>-0.47 | 03:50.46<br>03:53.11<br>1.15 | 04:12.56<br>04:12.21<br>-0.14 | 05:25.36<br>05:21.83<br>-1.08 | 08:06.11<br>08:15.15<br>1.86 | 14:28.09<br>14:12.19<br>-1.83 | 29:31.78<br>29:43.61<br>0.67  | 1.03      | 1:05:44.00<br>1:06:01.99<br>0.46  | 2:18:47.00<br>2:18:54.73<br>0.09  |
| 2002 | 05:25.36       | 372.42                 | 0.40           | 5.81           | 0.110           | 0.057           | 02:28.98<br>02:28.29<br>-0.47 | 03:50.46<br>03:53.11<br>1.15 | 04:12.56<br>04:12.21<br>-0.14 | 05:25.36<br>05:21.83<br>-1.08 | 08:06.11<br>08:15.15<br>1.86 | 14:28.09<br>14:12.19<br>-1.83 | 29:31.78<br>29:43.61<br>0.67  | 1.03      | 1:05:44.00<br>1:06:01.99<br>0.46  | 2:17:17.80<br>2:18:54.73<br>1.18  |
| 2003 | 05:25.36       | 372.42                 | 0.40           | 5.81           | 0.110           | 0.057           | 02:28.98<br>02:28.29<br>-0.47 | 03:50.46<br>03:53.11<br>1.15 | 04:12.56<br>04:12.21<br>-0.14 | 05:25.36<br>05:21.83<br>-1.08 | 08:06.11<br>08:15.15<br>1.86 | 14:28.09<br>14:12.19<br>-1.83 | 29:31.78<br>29:43.61<br>0.67  | 1.03      | 1:05:39.60<br>1:06:01.99<br>0.57  | 2:15:24.60<br>2:18:54.73<br>2.59  |
| 2004 | 05:25.36       | 372.59                 | 0.40           | 5.91           | 0.109           | 0.056           | 02:28.98<br>02:28.31<br>-0.45 | 03:50.46<br>03:53.06<br>1.13 | 04:12.56<br>04:12.14<br>-0.17 | 05:25.36<br>05:21.67<br>-1.13 | 08:06.11<br>08:14.78<br>1.78 | 14:24.68<br>14:11.28<br>-1.55 | 29:31.78<br>29:40.80<br>0.51  | 0.96      | 1:05:39.60<br>1:05:53.35<br>0.35  | 2:15:24.60<br>2:18:31.32<br>2.30  |
| 2005 | 05:25.36       | 372.59                 | 0.40           | 5.91           | 0.109           | 0.056           | 02:28.98<br>02:28.31<br>-0.45 | 03:50.46<br>03:53.06<br>1.13 | 04:12.56<br>04:12.14<br>-0.17 | 05:25.36<br>05:21.67<br>-1.13 | 08:06.11<br>08:14.78<br>1.78 | 14:24.68<br>14:11.28<br>-1.55 | 29:31.78<br>29:40.80<br>0.51  | 0.96      | 1:05:39.60<br>1:05:53.35<br>0.35  | 2:15:24.60<br>2:18:31.32<br>2.30  |
| 2006 | 05:25.36       | 372.60                 | 0.40           | 5.91           | 0.109           | 0.056           | 02:28.98<br>02:28.31<br>-0.45 | 03:50.46<br>03:53.06<br>1.13 | 04:12.56<br>04:12.14<br>-0.17 | 05:25.36<br>05:21.66<br>-1.14 | 08:06.11<br>08:14.77<br>1.78 | 14:24.53<br>14:11.24<br>-1.54 | 29:31.78<br>29:40.68<br>0.50  | 0.96      | 1:05:39.60<br>1:05:52.97<br>0.34  | 2:15:24.60<br>2:18:30.30<br>2.29  |
| 2007 | 05:25.36       | 373.00                 | 0.39           | 6.15           | 0.107           | 0.055           | 02:28.98<br>02:28.38<br>-0.40 | 03:50.46<br>03:52.95<br>1.08 | 04:12.56<br>04:11.98<br>-0.23 | 05:25.36<br>05:21.28<br>-1.25 | 08:06.11<br>08:13.93<br>1.61 | 14:16.63<br>14:09.15<br>-0.87 | 29:31.78<br>29:34.32<br>0.14  | 0.80      | 1:05:39.60<br>1:05:33.58<br>-0.15 | 2:15:24.60<br>2:17:38.07<br>1.64  |
| 2008 | 05:25.36       | 373.29                 | 0.39           | 6.31           | 0.106           | 0.054           | 02:28.98<br>02:28.42<br>-0.37 | 03:50.46<br>03:52.87<br>1.05 | 04:12.56<br>04:11.86<br>-0.28 | 05:25.36<br>05:21.01<br>-1.34 | 08:06.11<br>08:13.35<br>1.49 | 14:11.15<br>14:07.72<br>-0.40 | 29:31.78<br>29:30.03<br>-0.10 | 0.72      | 1:05:39.60<br>1:05:20.64<br>-0.48 | 2:15:24.60<br>2:17:03.41<br>1.22  |
| 2009 | 05:25.36       | 373.29                 | 0.39           | 6.31           | 0.106           | 0.054           | 02:28.98<br>02:28.42<br>-0.37 | 03:50.46<br>03:52.87<br>1.05 | 04:12.56<br>04:11.86<br>-0.28 | 05:25.36<br>05:21.01<br>-1.34 | 08:06.11<br>08:13.35<br>1.49 | 14:11.15<br>14:07.72<br>-0.40 | 29:31.78<br>29:30.03<br>-0.10 | 0.72      | 1:05:39.60<br>1:05:20.64<br>-0.48 | 2:15:24.60<br>2:17:03.41<br>1.22  |
| 2010 | 05:25.36       | 373.29                 | 0.39           | 6.31           | 0.106           | 0.054           | 02:28.98<br>02:28.42<br>-0.37 | 03:50.46<br>03:52.87<br>1.05 | 04:12.56<br>04:11.86<br>-0.28 | 05:25.36<br>05:21.01<br>-1.34 | 08:06.11<br>08:13.35<br>1.49 | 14:11.15<br>14:07.72<br>-0.40 | 29:31.78<br>29:30.03<br>-0.10 | 0.72      | 1:05:39.60<br>1:05:20.64<br>-0.48 | 2:15:24.60<br>2:17:03.41<br>1.22  |
| 2011 | 05:25.36       | 373.29                 | 0.39           | 6.31           | 0.106           | 0.054           | 02:28.98<br>02:28.42<br>-0.37 | 03:50.46<br>03:52.87<br>1.05 | 04:12.56<br>04:11.86<br>-0.28 | 05:25.36<br>05:21.01<br>-1.34 | 08:06.11<br>08:13.35<br>1.49 | 14:11.15<br>14:07.72<br>-0.40 | 29:31.78<br>29:30.03<br>-0.10 | 0.72      | 1:05:39.60<br>1:05:20.64<br>-0.48 | 2:15:24.60<br>2:17:03.41<br>1.22  |
| 2012 | 05:25.36       | 373.29                 | 0.39           | 6.31           | 0.106           | 0.054           | 02:28.98<br>02:28.42<br>-0.37 | 03:50.46<br>03:52.87<br>1.05 | 04:12.56<br>04:11.86<br>-0.28 | 05:25.36<br>05:21.01<br>-1.34 | 08:06.11<br>08:13.35<br>1.49 | 14:11.15<br>14:07.72<br>-0.40 | 29:31.78<br>29:30.03<br>-0.10 | 0.72      | 1:05:39.60<br>1:05:20.64<br>-0.48 | 2:15:24.60<br>2:17:03.41<br>1.22  |
| 2013 | 05:25.36       | 373.29                 | 0.39           | 6.31           | 0.106           | 0.054           | 02:28.98<br>02:28.42<br>-0.37 | 03:50.46<br>03:52.87<br>1.05 | 04:12.56<br>04:11.86<br>-0.28 | 05:25.36<br>05:21.01<br>-1.34 | 08:06.11<br>08:13.35<br>1.49 | 14:11.15<br>14:07.72<br>-0.40 | 29:31.78<br>29:30.03<br>-0.10 | 0.72      | 1:05:39.60<br>1:05:20.64<br>-0.48 | 2:15:24.60<br>2:17:03.41<br>1.22  |
| 2014 | 05:25.36       | 373.29                 | 0.39           | 6.31           | 0.106           | 0.054           | 02:28.98<br>02:28.42<br>-0.37 | 03:50.46<br>03:52.87<br>1.05 | 04:12.56<br>04:11.86<br>-0.28 | 05:25.36<br>05:21.01<br>-1.34 | 08:06.11<br>08:13.35<br>1.49 | 14:11.15<br>14:07.72<br>-0.40 | 29:31.78<br>29:30.03<br>-0.10 | 0.72      | 1:05:12.00<br>1:05:20.64<br>0.22  | 2:15:24.60<br>2:17:03.41<br>1.22  |
| 2015 | 05:25.36       | 373.37                 | 0.39           | 6.28           | 0.106           | 0.054           | 02:28.98<br>02:28.35<br>-0.42 | 03:50.07<br>03:52.79<br>1.18 | 04:12.56<br>04:11.78<br>-0.31 | 05:25.36<br>05:20.93<br>-1.36 | 08:06.11<br>08:13.26<br>1.47 | 14:11.15<br>14:07.66<br>-0.41 | 29:31.78<br>29:30.17<br>-0.09 | 0.75      | 1:05:09.00<br>1:05:21.63<br>0.32  | 2:15:24.60<br>2:17:07.00<br>1.26  |
| 2016 | 05:25.36       | 372.98                 | 0.40           | 7.21           | 0.108           | 0.051           | 02:28.98<br>02:28.29<br>-0.47 | 03:50.07<br>03:52.89<br>1.23 | 04:12.56<br>04:11.93<br>-0.25 | 05:25.36<br>05:21.30<br>-1.25 | 08:06.11<br>08:12.97<br>1.41 | 14:11.15<br>14:05.18<br>-0.70 | 29:17.45<br>29:18.93<br>0.08  | 0.77      | 1:05:09.00<br>1:04:40.89<br>-0.72 | 2:15:24.60<br>2:15:07.52<br>-0.21 |
| 2017 | 05:23.75       | 373.91                 | 0.38           | 6.80           | 0.104           | 0.052           | 02:28.98<br>02:28.41<br>-0.39 | 03:50.07<br>03:52.69<br>1.14 | 04:12.56<br>04:11.64<br>-0.36 | 05:23.75<br>05:20.61<br>-0.97 | 08:06.11<br>08:12.16<br>1.24 | 14:11.15<br>14:04.60<br>-0.77 | 29:17.45<br>29:20.21<br>0.16  | 0.72      | 1:04:51.00<br>1:04:50.19<br>-0.02 | 2:15:24.60<br>2:15:40.86<br>0.20  |

| Year | t <sub>c</sub> | v <sub>m</sub> [m/min] | E <sub>s</sub> | E <sub>l</sub> | Y <sub>an</sub> | Y <sub>ae</sub> | 1000     | 1500     | 1609.34  | 2000     | 3000     | 5000     | 10 000   | av.err [%] | Halfmarathon | Marathon   |
|------|----------------|------------------------|----------------|----------------|-----------------|-----------------|----------|----------|----------|----------|----------|----------|----------|------------|--------------|------------|
| 2018 | 05:23.75       | 373.91                 | 0.38           | 6.80           | 0.104           | 0.052           | 02:28.98 | 03:50.07 | 04:12.56 | 05:23.75 | 08:06.11 | 14:11.15 | 29:17.45 | 0.72       | 1:04:51.00   | 2:15:24.60 |
|      |                |                        |                |                |                 |                 | 02:28.41 | 03:52.69 | 04:11.64 | 05:20.61 | 08:12.16 | 14:04.60 | 29:20.21 |            | 1:04:50.19   | 2:15:40.86 |
|      |                |                        |                |                |                 |                 | -0.39    | 1.14     | -0.36    | -0.97    | 1.24     | -0.77    | 0.16     |            | -0.02        | 0.20       |
| 2019 | 05:23.75       | 373.98                 | 0.38           | 6.76           | 0.104           | 0.052           | 02:28.98 | 03:50.07 | 04:12.33 | 05:23.75 | 08:06.11 | 14:11.15 | 29:17.45 | 0.71       | 1:04:51.00   | 2:14:04.00 |
|      |                |                        |                |                |                 |                 | 02:28.38 | 03:52.65 | 04:11.59 | 05:20.54 | 08:12.09 | 14:04.55 | 29:20.32 |            | 1:04:51.04   | 2:15:43.91 |
|      |                |                        |                |                |                 |                 | -0.40    | 1.12     | -0.29    | -0.99    | 1.23     | -0.78    | 0.16     |            | 0.00         | 1.24       |
| 2020 | 05:23.75       | 374.22                 | 0.38           | 6.93           | 0.103           | 0.052           | 02:28.98 | 03:50.07 | 04:12.33 | 05:23.75 | 08:06.11 | 14:06.62 | 29:17.45 | 0.63       | 1:04:31.00   | 2:14:04.00 |
|      |                |                        |                |                |                 |                 | 02:28.42 | 03:52.58 | 04:11.50 | 05:20.32 | 08:11.61 | 14:03.37 | 29:16.79 |            | 1:04:40.42   | 2:15:15.63 |
|      |                |                        |                |                |                 |                 | -0.37    | 1.09     | -0.33    | -1.06    | 1.13     | -0.38    | -0.04    |            | 0.24         | 0.89       |
| 2021 | 05:21.56       | 375.02                 | 0.37           | 7.58           | 0.100           | 0.049           | 02:28.98 | 03:50.07 | 04:12.33 | 05:21.56 | 08:06.11 | 14:06.62 | 29:01.03 | 0.60       | 1:02:52.00   | 2:14:04.00 |
|      |                |                        |                |                |                 |                 | 02:28.51 | 03:52.44 | 04:11.28 | 05:19.80 | 08:10.17 | 13:59.75 | 29:05.70 |            | 1:04:06.71   | 2:13:45.50 |
|      |                |                        |                |                |                 |                 | -0.32    | 1.03     | -0.42    | -0.55    | 0.84     | -0.81    | 0.27     |            | 1.98         | -0.23      |
| 2022 | 05:21.56       | 375.02                 | 0.37           | 7.58           | 0.100           | 0.049           | 02:28.98 | 03:50.07 | 04:12.33 | 05:21.56 | 08:06.11 | 14:06.62 | 29:01.03 | 0.60       | 1:02:52.00   | 2:14:04.00 |
|      |                |                        |                |                |                 |                 | 02:28.51 | 03:52.44 | 04:11.28 | 05:19.80 | 08:10.17 | 13:59.75 | 29:05.70 |            | 1:04:06.71   | 2:13:45.50 |
|      |                |                        |                |                |                 |                 | -0.32    | 1.03     | -0.42    | -0.55    | 0.84     | -0.81    | 0.27     |            | 1.98         | -0.23      |
| 2023 | 05:21.56       | 377.10                 | 0.36           | 6.93           | 0.098           | 0.052           | 02:28.98 | 03:49.11 | 04:07.64 | 05:21.56 | 08:06.11 | 14:00.21 | 29:01.03 | 0.66       | 1:02:52.00   | 2:11:53.00 |
|      |                |                        |                |                |                 |                 | 02:27.90 | 03:51.22 | 04:09.92 | 05:17.86 | 08:07.84 | 13:56.92 | 29:03.39 |            | 1:04:10.90   | 2:14:14.08 |
|      |                |                        |                |                |                 |                 | -0.72    | 0.92     | 0.92     | -1.15    | 0.36     | -0.39    | 0.14     |            | 2.09         | 1.78       |
